# Supplementary material for: Restoration of User Videos Shared on Social Media
Source: arXiv:2208.08597 source file (2022-08-26)
Supplement: Supplementary file 1 [file Supplementary_material.pdf]

# Restoration of User Videos Shared on Social Media

Hongming Luo, Fei Zhou, Kin-Man Lam, Guoping Qiu

## 1 USER VIDEOS SHARED ON SOCIAL MEDIA DATASET

More information about the UVSSM dataset is shown in Table 1 and some examples are shown in Figure 1.

Table 1. Information about the UVSSM dataset

| | WeChat | Twitter | Bilibili | YouTube |
|---|---|---|---|---|
| Original res. | 1920 × 1080 | 1280 × 720 | 1280 × 720 | 1280 × 720 |
| Shared res. | 960 × 540 | 640 × 360 | 640 × 360 | 640 × 360 |
| No. of video | 214 | 50 | 50 | 50 |
| Default no. of train set | 200 | 40 | 40 | 40 |
| Default no. of validation set | 4 | 0 | 0 | 0 |
| Default no. of test set | 10 | 10 | 10 | 10 |
| No. of frames (per video) | 100 | 100 | 100 | 100 |

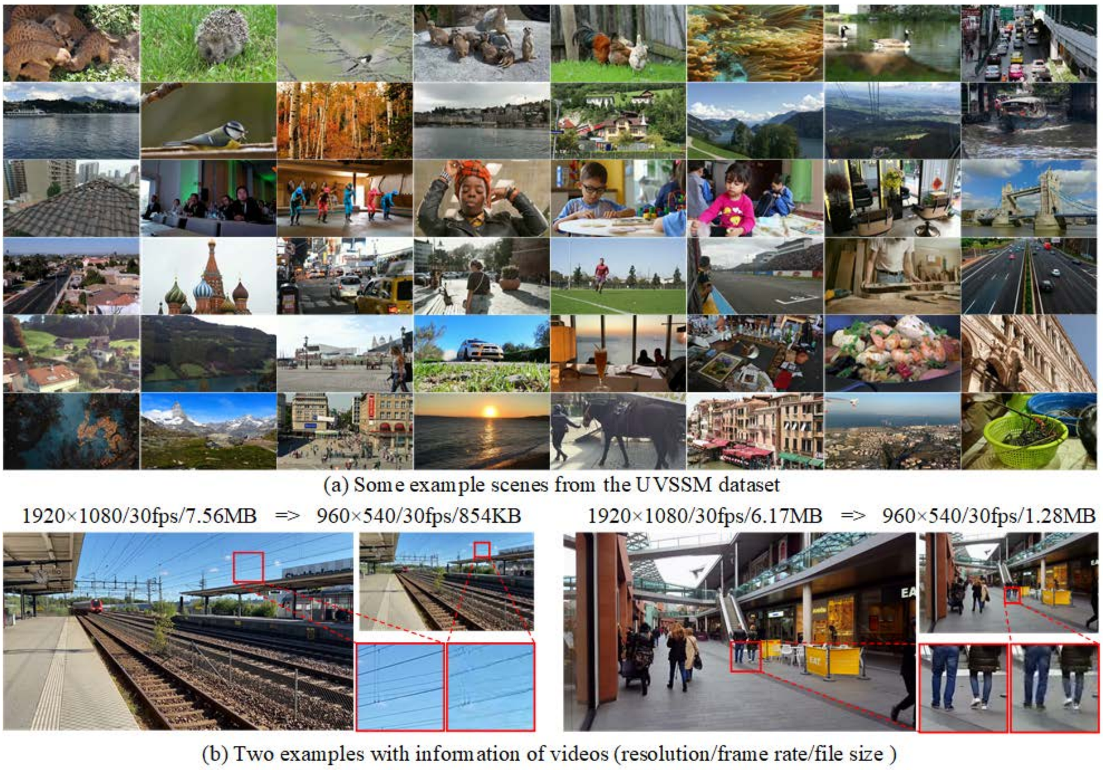


Figure 1. Some examples from the UVSSM dataset. In (b), The left frame in each example is from original videos and the top right one is from shared videos. The information above two examples represents the file information from original videos to shared videos.

**Data Collection**. The high quality (HQ) videos in UVSSM are directly from mobile phone

cameras and from the Internet, including Flickr.com, Vimeo.com, videvo.net and YouTube.com. Specifically, 100 videos are from camera phones and the remaining videos are from the Internet. The spatial resolutions of these original videos are either 1920 × 1080 or 1280 × 720 in high quality H.264 format and YUV 4:2:0. All source videos UVSSM dataset have the Creative Commons Attribution license (reuse allowed). Note that the UVSSM dataset is only for academic and research proposes, and we will make this explicit when release the data.

**Diversity.** The content diversity of the UVSSM dataset are as follows. As shown in Figure 2, the UVSSM dataset contains seven categories of scenes, *i.e.*, city, scenery, vehicle, animal, human, indoor, and object. Of the 264 videos, 47 contain fast motion. Additionally, for 62 videos, the camera is slightly shaky (*e.g.*, captured by handheld camera). Besides, 18 videos are in dark environments, *e.g.*, at night or underwater with insufficient lighting. The diversity of UVSSM is similar to that of other video restoration dataset, *e.g.*, NTIRE2021 [9].

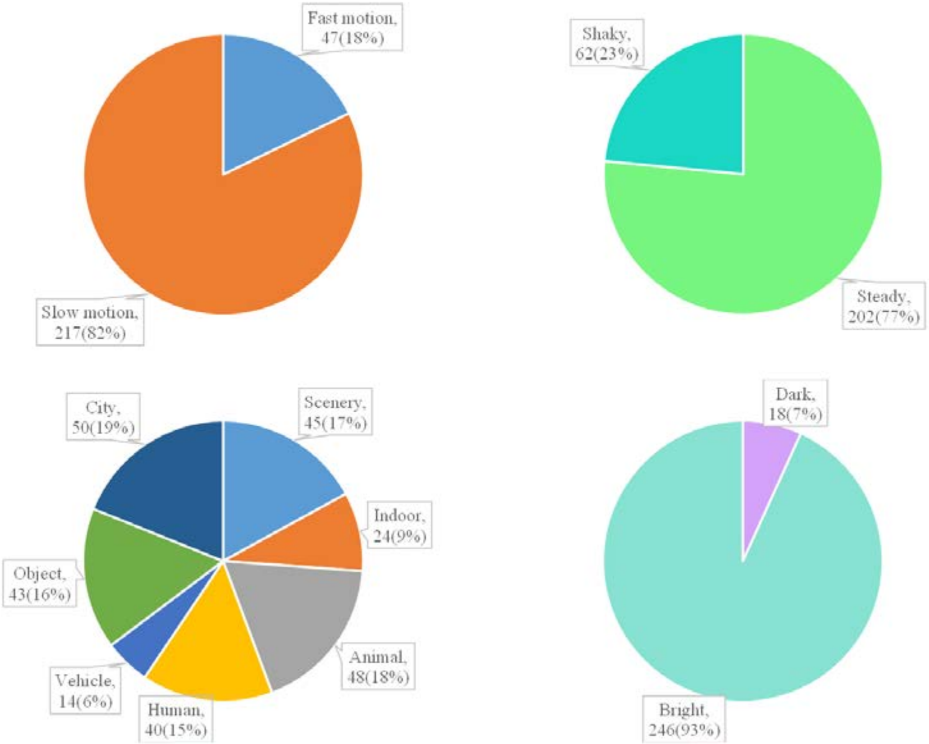


Figure 2. The diversity of the proposed UVSSM dataset.

**Degradation and Partition.** To collect the degraded videos, we have used five different brands of mobile phone including Apple, Samsung, Huawei, Xiaomi, and Oneplus to share 214 videos with a resolution of 1920 × 1080 on WeChat. The transmitted videos have a resolution of 960 × 540 and lower qualities. In addition to WeChat, we have uploaded 50 videos that are not included in the 214 shared on WeChat to each of the three other platforms, *i.e.*, Twitter, Bilibili, and YouTube, and downloaded a 640 × 360 version of these videos. Therefore, the UVSSM dataset contains a total of 364 pairs of original and shared videos (214 WeChat, 50 Bilibili, 50 Twitter and 50 YouTube).

# 2 EXPERIMENTS

## 2.1 Implementation Details

The Feature Extraction Alignment Module (FEAM) in our model is similar to the Pyramid Cascaded Deformable network (PCD) in EDVR [8]. The details of the PCD module are shown in Figure 3. We take 5 frames $\mathbf{x} = \{\mathbf{x}_{t-2}, \mathbf{x}_{t-1}, \mathbf{x}_t, \mathbf{x}_{t+1}, \mathbf{x}_{t+2}\}$ as input. The PCD module is used to align the neighboring frames $\{\mathbf{x}_{t-2}, \mathbf{x}_{t-1}, \mathbf{x}_{t+1}, \mathbf{x}_{t+2}\}$ to the $t$-th frame and extract the features as:

$$F'_i = PCD(\mathbf{x}_t, \mathbf{x}_i), \; i = \{t-2, t-1, t+1, t+2\}, \quad (1)$$

where the $F'_i$ is the aligned features. After that, all aligned features are concatenated and passed to the next module as:

$$F' = concat(F'_{t-2}, F'_{t-1}, F_t, F'_{t+1}, F'_{t+2}), \quad (2)$$

where $F_t$ is the features of center frame that no need to be aligned.

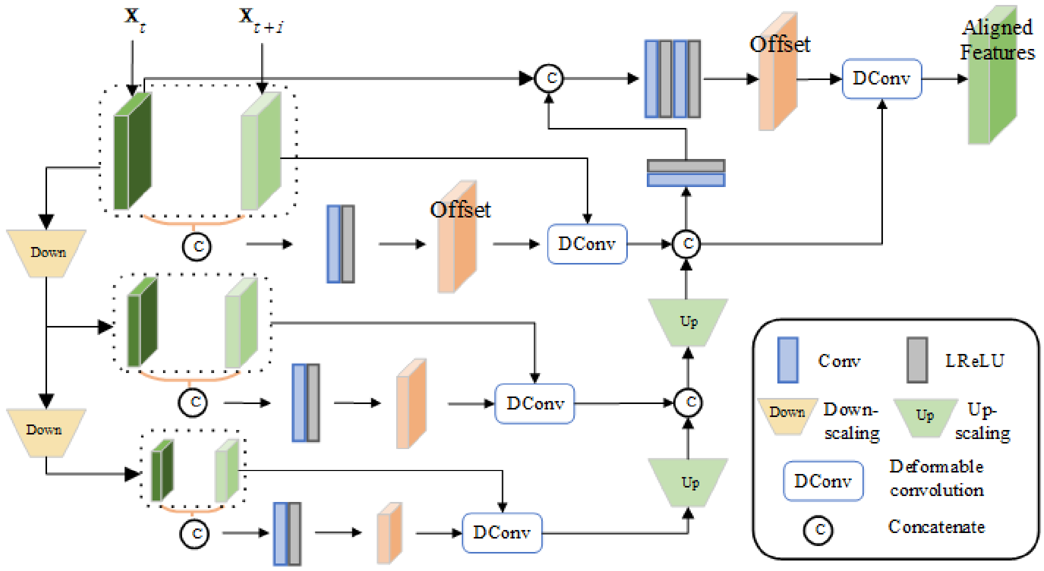


Figure 3. The architecture of the PCD alignment module.

The learnable network $\mathcal{F}_{B_1}$ and $\mathcal{F}_{B_2}$ in the degradation sensing module are implemented similar to the backbone network used in BIN [6]. The architecture of the backbone network is shown in Figure 4. The residual dense block (RDB) is adopted from the residual dense network of [10]. We use 6 RDBs in our model and the filters number is set as 64. The down-shuffle in Figure 4 is the reverse operation of up-shuffle, which is the same as the pixel shuffle operation in [7]. The scale of down-shuffle and up-shuffle is 2. Long skip connection is also adopted in the backbone network and features from each RDB are concatenated to the next convolutional layer.

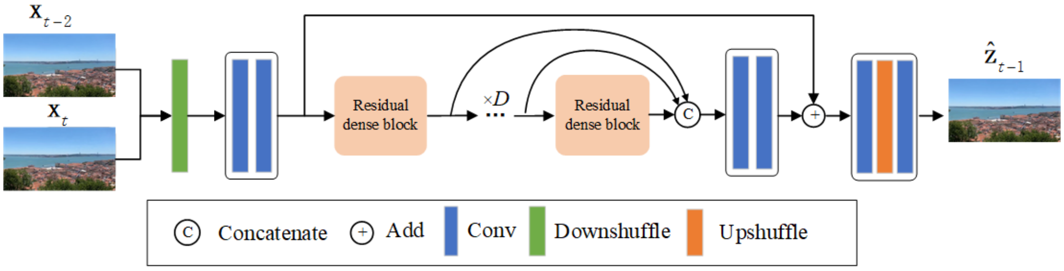


Figure 4. The architecture of the backbone in BIN model.

And there are more training details of other methods. We use bicubic down-scaling to scale the original videos the have the same resolution as that of the shared videos and refer them as LR uncompressed videos. We take the shared videos as input and LR uncompressed videos as target to train the STDF[2] model and the backbone network in our degradation sensing module. Then we take the output of the STDF model as input and original videos as target to train the SR models, *i.e.*, EDVR[8], RSDN[3], VSRTGA[4] and BasicVSR[1]. As for the COMISR[5] and the second stage training of our model, we take the shared videos as input and the original videos as target.

## 2.2 More Visual Comparison of Results

More visual comparisons are shown in Figure 5, 6, 7, and 8. From these visual comparisons, we can see that our method achieves the best restoration against other methods.

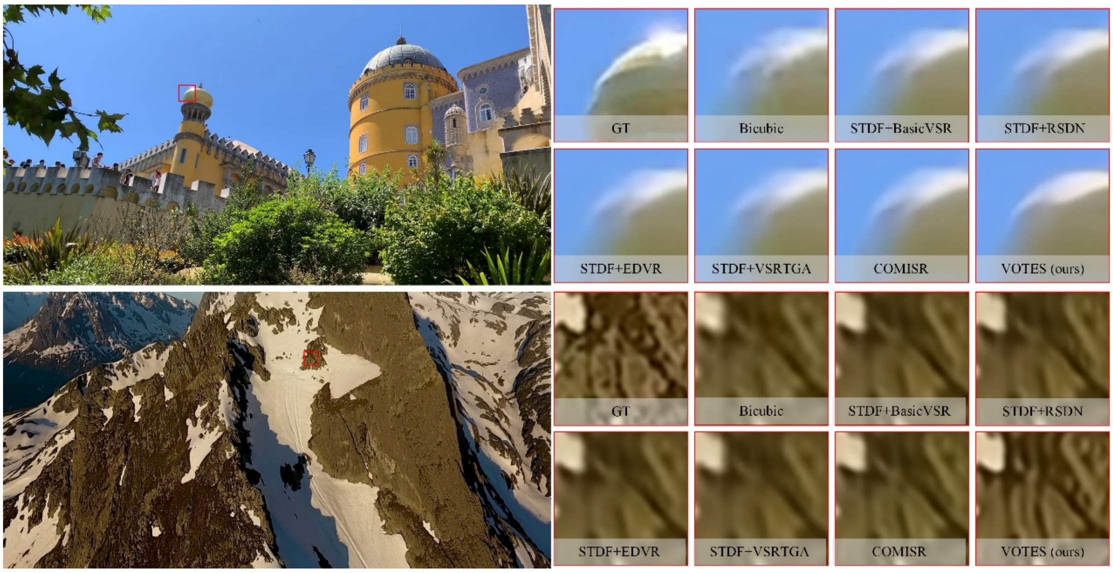


Figure 5. The visual comparison on UVSSM (scale factor: 2).

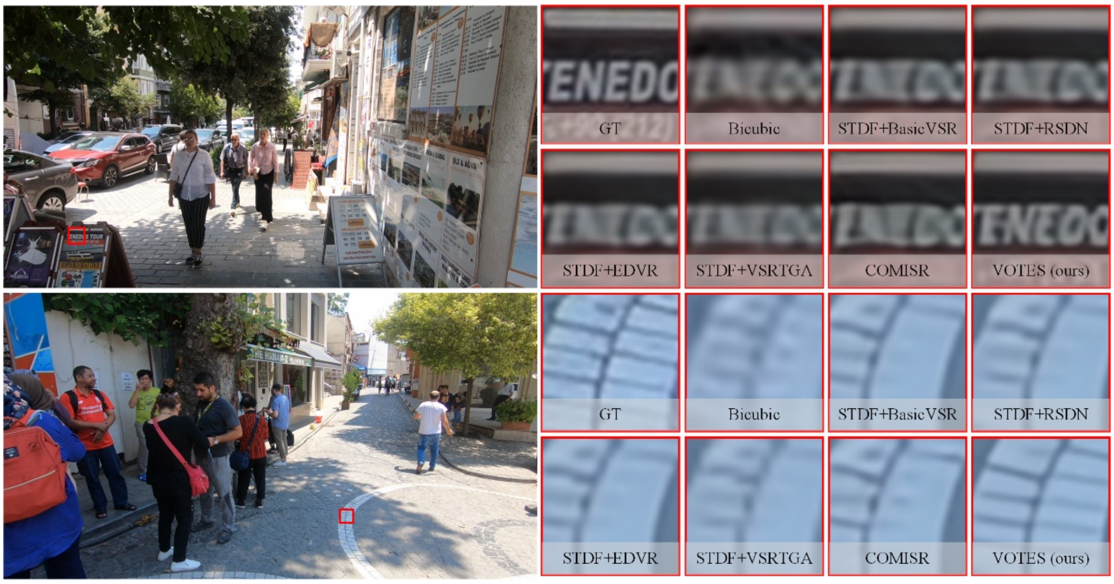


Figure 6. The visual comparison on REDS [11] (QP: 33, scale factor: 2).

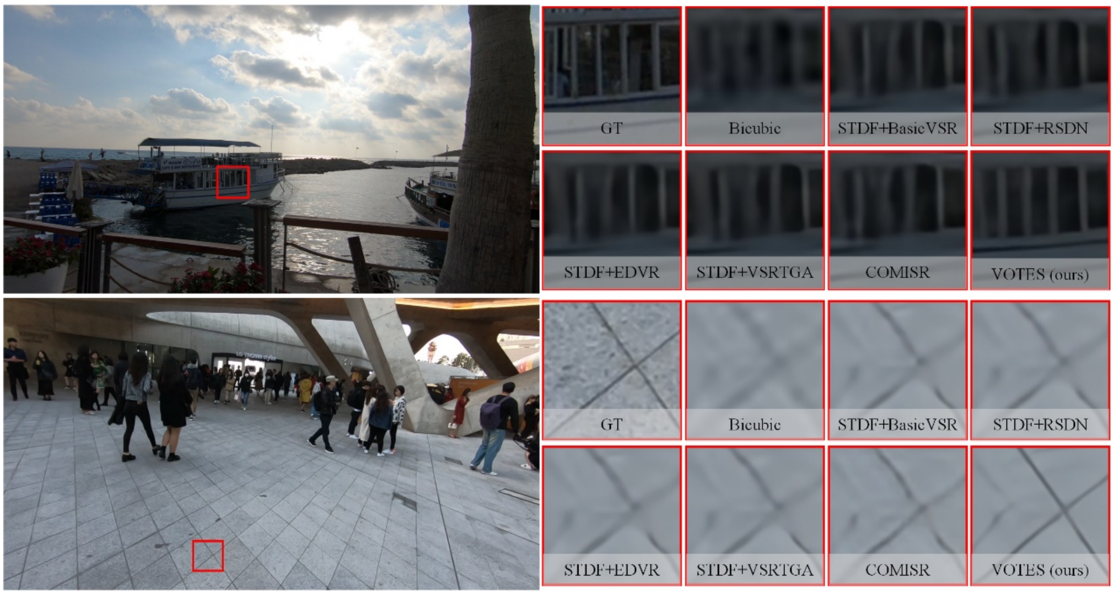


Figure 7. The visual comparison on REDS (QP: 28, scale factor: 4).

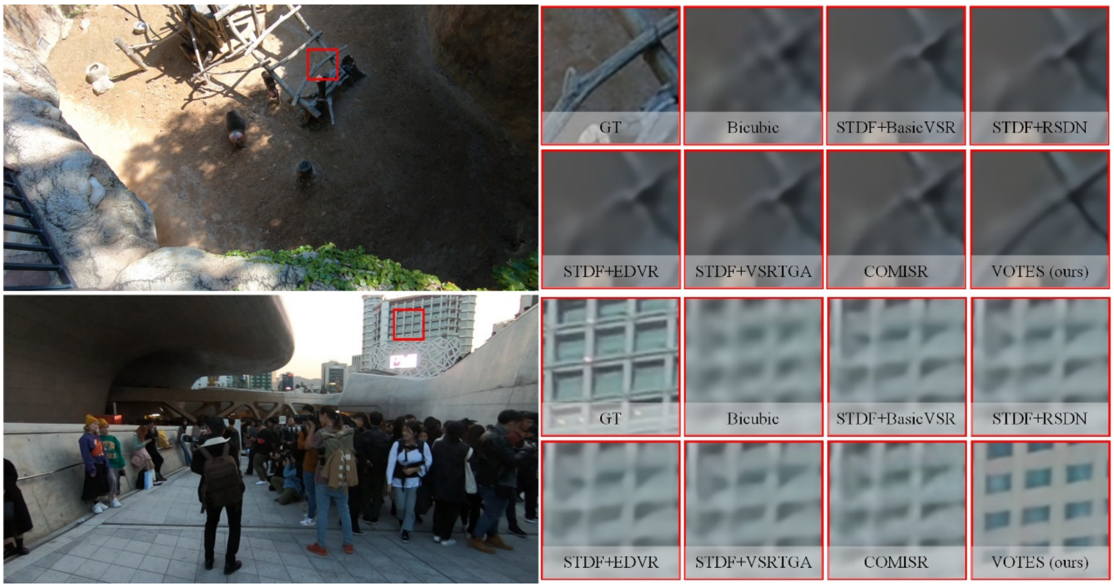


Figure 8. The visual comparison on REDS (QP: 33, scale factor: 4).

## 2.3 More Examples of How the DFM Relates to Restoration Errors

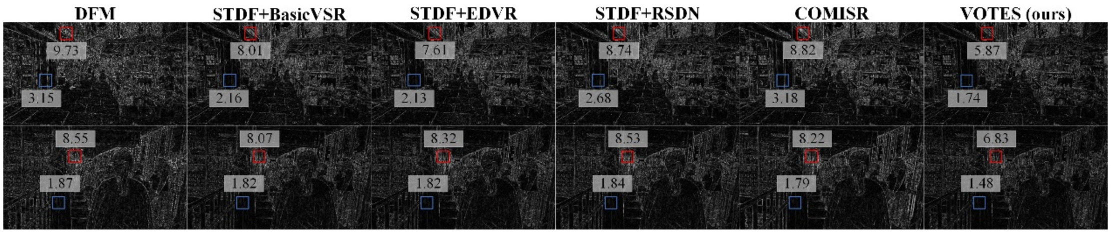


Figure 9. Relation between DFM and restoration errors. The DFMs are in the 1st column, the rest are actual restoration error of different methods. The number above each red box is the average element value within the red box. Note the original resolution of the DFM is half of that of the actual restoration error maps, it is resized here for visualization convenience. Data from the REDS dataset and QP = 33, scaling factor = 2.

## 2.4 More Results

We have also implemented other video super-resolution (VSR) models compared in the paper by using the shared video as input and the original as target for data shared on WeChat. Results are shown in Table. 2. From these results, we can see that our model also consistently outperforms other SOTA VSR models. Figure 10 shows visual examples of this implementation scheme, again it is seen that our new method has achieved better results.

Table 2. Quantitative comparison of performances (PSNR (dB)/SSIM). **Blod** text indicates the best performance.

| Clip number | A+[12] | EDVR | RSDN | VSRTGA | BasicVSR | VOTES(ours) |
|---|---|---|---|---|---|---|
| 001 | 35.4/0.944 | 36.0/0.954 | 35..6/0.953 | 36.1/0.953 | 36.0/0.953 | **37.2/0.959** |
| 002 | 31.3/0.896 | 33.6/**0.928** | 31.6/0.907 | 31.8/0.907 | 31.8/0.907 | **33.7/0.928** |
| 003 | 29.9/0.875 | 32.0/0.906 | 31.1/0.897 | 30.9/0.897 | 30.9/0.895 | **33.0/0.910** |
| 004 | 30.9/0.911 | 33.1/0.935 | 31.6/0.924 | 32.0/0.925 | 31.7/0.921 | **34.4/0.940** |
| 005 | 34.9/0.935 | 34.4/0.948 | 35.4/0.949 | 35.8/0.951 | 35.6/0.950 | **37.1/0.956** |
| 006 | 29.8/0.878 | 30.8/0.911 | 30.3/0.904 | 30.8/0.908 | 30.6/0.906 | **32.6/0.920** |
| 007 | 29.4/0.834 | 30.8/**0.873** | 30.0/0.860 | 30.1/0.858 | 30.1/0.858 | **31.1/0.873** |
| 008 | 27.1/0.772 | **28.5/0.814** | 27.6/0.795 | 27.7/0.797 | 27.6/0.792 | **28.5/0.814** |
| 009 | 29.7/0.846 | 29.9/0.858 | 29.2/0.856 | 30.1/0.858 | 30.1/0.859 | **30.3/0.861** |
| 010 | 34.2/0.920 | **36.2**/0.939 | 34.5/0.928 | 34.7/0.930 | 34.4/0.928 | 35.9/**0.940** |
| average | 31.2/0881 | 32.5/0.907 | 31.7/0.8997 | 32.0/0.898 | 31.9/0.897 | **33.4/0.910** |

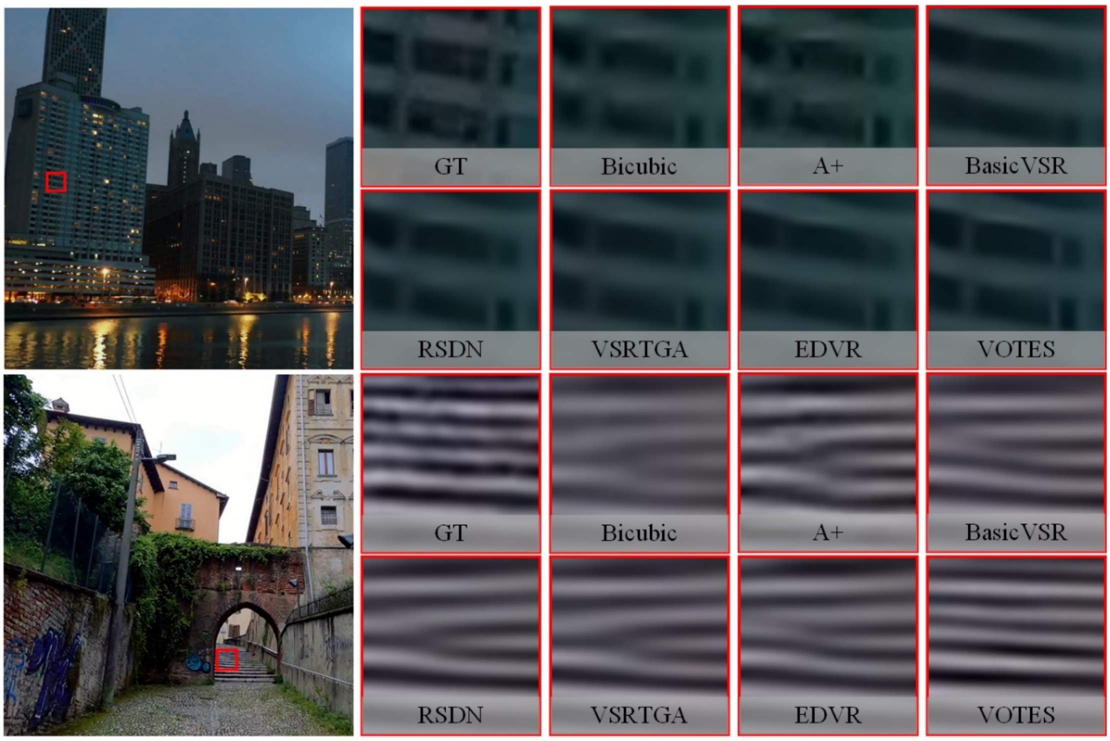


Figure 10. The visual comparison.

## REFERENCES


[1] Kelvin C.K. Chan, Xintao Wang, Ke Yu, Chao Dong, and Chen Change Loy. 2021. BasicVSR: The Search for Essential Components in Video Super-Resolution and Beyond. In 2021 IEEE/CVF Conference on Computer Vision and Pattern Recognition (CVPR). 4945–4954.

[2] Jianing Deng, Li Wang, Shiliang Pu, and Cheng Zhuo. 2020. Spatio-Temporal Deformable Convolution for Compressed Video Quality Enhancement. In Proceedings of the Conference on Artificial Intelligence, Vol. 34. 10696–10703.

[3] Takashi Isobe, Xu Jia, Shuhang Gu, Songjiang Li, Shengjin Wang, and Qi Tian. 2020. Video Super-resolution with Recurrent Structure-detail Network. In European Conference on Computer Vision. Springer, 645–660.

[4] Takashi Isobe, Songjiang Li, Xu Jia, Shanxin Yuan, Gregory Slabaugh, Chunjing Xu, Ya-Li Li, Shengjin Wang, and Qi Tian. 2020. Video Super-Resolution With Temporal Group Attention. In 2020 IEEE/CVF Conference on Computer Vision and Pattern Recognition (CVPR). 8005–8014.

[5] Yinxiao Li, Pengchong Jin, Feng Yang, Ce Liu, Ming-Hsuan Yang, and Peyman Milanfar. 2021. COMISR: Compression-Informed Video Super-Resolution. In 2021 IEEE/CVF International Conference on Computer Vision (ICCV). 2523–2532.

[6] Wang Shen, Wenbo Bao, Guangtao Zhai, Li Chen, Xiongkuo Min, and Zhiyong Gao. 2020. Blurry Video Frame Interpolation. In 2020 IEEE/CVF Conference on Computer Vision and Pattern Recognition (CVPR). 5113–5122.

[7] Wenzhe Shi, Jose Caballero, Ferenc Huszár, Johannes Totz, Andrew P. Aitken, Rob Bishop, Daniel Rueckert, and Zehan Wang. 2016. Real-Time Single Image and Video Super-Resolution Using an Efficient Sub-Pixel Convolutional Neural Network. In 2016 IEEE Conference on Computer Vision and Pattern Recognition (CVPR). 1874–1883.

[8] Xintao Wang, Kelvin C.K. Chan, Ke Yu, Chao Dong, and Chen Change Loy. 2019. EDVR: Video Restoration With Enhanced Deformable Convolutional Networks. In 2019 IEEE/CVF Conference on Computer Vision and Pattern Recognition Workshops (CVPRW). 1954–1963.

[9] Ren Yang and Radu Timofte. 2021. NTIRE 2021 Challenge on Quality Enhancement of Compressed Video: Dataset and Study. In 2021 IEEE/CVF Conference on Computer Vision and Pattern Recognition Workshops (CVPRW). 667–676.

[10] Yulun Zhang, Yapeng Tian, Yu Kong, Bineng Zhong, and Yun Fu. 2018. Residual Dense Network for Image Super-Resolution. In 2018 IEEE/CVF Conference on Computer Vision and Pattern Recognition (CVPR). 2472–2481.

[11] Seungjun Nah, Sungyong Baik, Seokil Hong, Gyeongsik Moon, Sanghyun Son, Radu Timofte, and Kyoung Mu Lee. 2019. NTIRE 2019 Challenge on Video Deblurring and Super-Resolution: Dataset and Study. In 2019 IEEE/CVF Conference on Computer Vision and Pattern Recognition Workshops (CVPRW). 1996–2005.

[12] Radu Timofte, Vincent De Smet, and Luc Van Gool. 2014. A+: Adjusted Anchored Neighborhood Regression for Fast Super-Resolution. In 2014 Asian Conference on Computer Vision (ACCV). 111-126.
